# Supplementary material for: Layout-Corrector: Alleviating Layout Sticking Phenomenon in Discrete Diffusion Model
Source: arXiv:2409.16689 source file (2024-09-25)
Supplement: Supplementary file 2 [file vs_sota_crello.tex]

\begin{table*}[t]
\caption{Comparison with SoTA models for the three tasks on Crello dataset~\cite{yamaguchi2021canvasvae}. * indicates that the model was designed for conditional generation, thus results of unconditional task are omitted. Best and second-best results are in \textbf{bold} and with {\ul underline}, respectively.}
\label{tab:vs_sota_crello}
\centering
\begin{tabular}{llrrrrrr}
\toprule
 & Task & \multicolumn{2}{c}{Unconditional} & \multicolumn{2}{c}{C$\rightarrow$S+P} & \multicolumn{2}{c}{C+S$\rightarrow$P} \\ 
\cmidrule(r){2-2} \cmidrule(lr){3-4} \cmidrule(lr){5-6} \cmidrule(l){7-8}
Model & Type & \multicolumn{1}{c}{FID$\downarrow$} & \multicolumn{1}{c}{Align.$\rightarrow$} &  \multicolumn{1}{c}{FID$\downarrow$} & \multicolumn{1}{c}{Max-IoU$\uparrow$} & \multicolumn{1}{c}{FID$\downarrow$} & \multicolumn{1}{c}{Max-IoU$\uparrow$}  \\
\cmidrule(r){1-1} \cmidrule(lr){2-2} \cmidrule(lr){3-3} \cmidrule(lr){4-4} \cmidrule(lr){5-5} \cmidrule(lr){6-6} \cmidrule(lr){7-7} \cmidrule(lr){8-8} 
DLT~\cite{levi2023dlt} & Continuous & {\ul 4.71} & 0.484 & 4.29 & \textbf{0.212} & 3.68 & \textbf{0.278} \\

BLT*~\cite{kong2022blt} & Discrete   & - & - & 18.3 & 0.199 & 5.12 & {\ul 0.259} \\
LayoutTrans~\cite{gupta2021layouttransformer} & Discrete & 5.93 & \textbf{0.305} & 6.42 & {\ul 0.203} & 3.87 & 0.258 \\
LayoutDM~\cite{inoue2023layoutdm} & Discrete & 5.28 & {\ul 0.280} & {\ul 4.04} & 0.197 & {\ul 3.55} & 0.248 \\ 
\rowcolor[HTML]{EFEFEF} 
\begin{tabular}[c]{@{}l@{}}\textbf{LayoutDM}~\cite{inoue2023layoutdm}\\ \textbf{+ Corrector (Ours)}\end{tabular} & Discrete & \textbf{4.59} & 0.227 & \textbf{3.44} & 0.202 & \textbf{3.30} & 0.254 \\ 
\cmidrule(r){1-1} \cmidrule(lr){2-2} \cmidrule(lr){3-3} \cmidrule(lr){4-4} \cmidrule(lr){5-5} \cmidrule(lr){6-6} \cmidrule(lr){7-7} \cmidrule(lr){8-8} 
\textit{Real data} & & 2.32 & 0.338 & 2.32 & 0.301 & 2.32 & 0.301 \\ \bottomrule
\end{tabular}
\end{table*}
