# Supplementary material for: Layout-Corrector: Alleviating Layout Sticking Phenomenon in Discrete Diffusion Model
Source: arXiv:2409.16689 source file (2024-09-25)
Supplement: Supplementary file 4 [file baseline_plus_cor_category_to_size_plus_position.tex]

\centering
\resizebox{\textwidth}{!}{%
\begin{tabular}{llccccccccc}
\toprule
                                  &        & \multicolumn{3}{c}{Rico~\cite{deka2017rico}}             & \multicolumn{3}{c}{PubLayNet~\cite{zhong2019publaynet}}  & \multicolumn{3}{c}{Crello~\cite{yamaguchi2021canvasvae}} \\ \cmidrule(r){3-5} \cmidrule(lr){6-8} \cmidrule(l){9-11}
Model                             & Arch.  & FID$\downarrow$ & Density$\uparrow$ & Coverage$\uparrow$ & FID$\downarrow$ & Density$\uparrow$ & Coverage$\uparrow$ & FID            & Density$\uparrow$  & Coverage$\uparrow$ \\ \cmidrule(r){1-1} \cmidrule(lr){2-2} \cmidrule(lr){3-3} \cmidrule(lr){4-4} \cmidrule(lr){5-5} \cmidrule(lr){6-6} \cmidrule(lr){7-7} \cmidrule(lr){8-8} \cmidrule(lr){9-9} \cmidrule(lr){10-10} \cmidrule(r){11-11}
MaskGIT~\cite{chang2022maskgit}   & Non-AR & 28.9            & 0.636             & 0.536              & 17.5            & 0.270             & 0.458              & 31.8           & 0.744              & 0.510              \\
\rowcolor[HTML]{EFEFEF} 
\textbf{~~+ Corrector}              &        & \textbf{17.3}   & 0.449             & \textbf{0.648}     & 22.1            & 0.155             & 0.357              & \textbf{11.6}  & 0.524              & \textbf{0.643}     \\
\rowcolor[HTML]{E6E6E6} 
\textbf{~~+ Corrector$^{\dagger}$}  &        & \textbf{10.5}   & 0.596             & \textbf{0.715}     & \textbf{15.7}   & 0.239             & \textbf{0.476}     & \textbf{5.73}  & 0.596              & \textbf{0.708}     \\ \cmidrule(r){1-1} \cmidrule(lr){2-2} \cmidrule(lr){3-3} \cmidrule(lr){4-4} \cmidrule(lr){5-5} \cmidrule(lr){6-6} \cmidrule(lr){7-7} \cmidrule(lr){8-8} \cmidrule(lr){9-9} \cmidrule(lr){10-10} \cmidrule(r){11-11}
VQDiffusion~\cite{gu2022vector}   & DDMs   & 3.90            & 0.610             & 0.771              & 7.73            & 0.334             & 0.592              & 4.30           & 0.566              & 0.728              \\
\rowcolor[HTML]{EFEFEF} 
\textbf{~~+ Corrector}              &        & \textbf{2.64}   & \textbf{0.700}    & \textbf{0.799}     & \textbf{5.45}   & \textbf{0.462}    & \textbf{0.679}     & \textbf{3.86}  & \textbf{0.685}     & \textbf{0.764}     \\
\rowcolor[HTML]{E6E6E6} 
\textbf{~~+ Corrector$^{\dagger}$}  &        & \textbf{2.65}   & \textbf{0.704}    & \textbf{0.803}     & \textbf{5.48}   & \textbf{0.465}    & \textbf{0.682}     & \textbf{4.03}  & \textbf{0.671}     & \textbf{0.760}     \\ \cmidrule(r){1-1} \cmidrule(lr){2-2} \cmidrule(lr){3-3} \cmidrule(lr){4-4} \cmidrule(lr){5-5} \cmidrule(lr){6-6} \cmidrule(lr){7-7} \cmidrule(lr){8-8} \cmidrule(lr){9-9} \cmidrule(lr){10-10} \cmidrule(r){11-11}
LayoutDM~\cite{inoue2023layoutdm} & DDMs   & 3.51            & 0.641             & 0.787              & 7.94            & 0.307             & 0.557              & 4.04           & 0.577              & 0.741              \\
\rowcolor[HTML]{EFEFEF} 
\textbf{~~+ Corrector}              &        & \textbf{2.43}   & \textbf{0.730}    & \textbf{0.807}     & \textbf{5.75}   & \textbf{0.438}    & \textbf{0.657}     & \textbf{3.44}  & \textbf{0.671}     & \textbf{0.769}     \\ \bottomrule
\end{tabular}
}
\caption{C $\rightarrow$ S $+$ P task}
\label{tab:base_plus_cor_category_to_size_plus_position}
